# Supplementary material for: Monotone function estimation in the presence of extreme data coarsening: Analysis of preeclampsia and birth weight in urban Uganda
Source: arXiv:1912.06946 source file (2019-12-14)
Supplement: Supplementary file 2 [file 08-appendix.tex]

%!TEX root = ../mulago-paper.tex

%---------------------------------------------------------

APPENDIX
